# Supplementary material for: Dynamics and Contracts for an Agent with Misspecified Beliefs
Source: arXiv:2405.20423 source file (2024-05-30)
Supplement: Supplementary file 1 [file convergence_two_actions.tex]

\section{Missing Proofs for Convergence to Berk-Nash for a Learning Agent with Two Actions}\label{apx:convergence two actions}
