# Supplementary material for: Dynamics and Contracts for an Agent with Misspecified Beliefs
Source: arXiv:2405.20423 source file (2024-05-30)
Supplement: Supplementary file 2 [file ergodic_divergence.tex]

\subsection{Missing Proofs for Ergodic Divergence}
\label{apx:ergodic divergence}
